# Supplementary material for: Robust electronic and tunable magnetic states in Sm$ _{2} $NiMnO$ _{6} $ ferromagnetic insulator
Source: arXiv:2204.08843 source file (2022-04-19)
Supplement: Supplementary file 1 [file Supplementary_Informations_SNMO_film_E_V2.tex]

\documentclass[12pt]{iopart}%{revtex4}%{iopart}%{article} 
%\documentclass[twocolumn,superscriptaddress,floatfix,preprintnumbers]{revtex4}
%\newcommand{\gguide}{{\it Preparing graphics for IOP Publishing journals}}
%Uncomment next line if AMS fonts required
%\usepackage{iopams} 
%\usepackage{amssymb}
\usepackage{graphicx}
\usepackage{multirow}
\usepackage{booktabs,siunitx}

\begin{document}

\title[]{Supplementary Information: \\ Robust electronic and tunable magnetic states in Sm$ _{2} $NiMnO$ _{6} $ ferromagnetic insulator}

\author{
S. Majumder$^{a}$,
\
M. Tripathi$^{a}$,
\
I. P\'{i}\v{s}$^{b,c}$,
\
S. Nappini$^{c}$,
\
P. Rajput$^{d}$,
\
S. N. Jha$^{d}$,
\
R. J. Choudhary$^{a}$,
and
D. M. Phase$^{a}$
\\
$^{a}$UGC DAE Consortium for Scientific Research, Indore 452001, India\\
$^{b}$Elettra Sicrotrone Trieste S.C.p.A., S.S. 14-km 163.5, 34149 Basovizza, Trieste, Italy\\
$^{c}$IOM CNR, Laboratorio TASC, S.S. 14-km 163.5, 34149 Basovizza, Trieste, Italy\\
$^{d}$Beamline Development and Application Section, Bhabha Atomic Research Centre, Mumbai 400085, India\\}
\ead{$^{*}$ram@csr.res.in}

\begin{figure*}[h!]\renewcommand{\thefigure}{S\arabic{figure}}
\centering
\includegraphics[angle=0,width=1.0\textwidth]{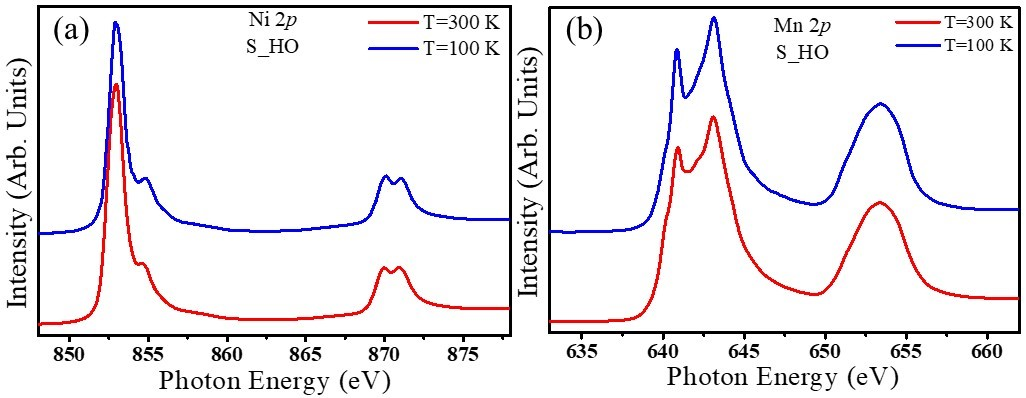}
\caption{Experimentally observed photo absorption spectra measured for S$\_$HO sample at T=300 K, 100 K across (a): Ni and (b): Mn \textit{L}$ _{3,2} $ edges. To have better visualization spectra are vertically translated here.}\label{xasvstem}
\end{figure*}

\begin{figure*}[]\renewcommand{\thefigure}{S\arabic{figure}}
\centering
\includegraphics[angle=0,width=0.5\textwidth]{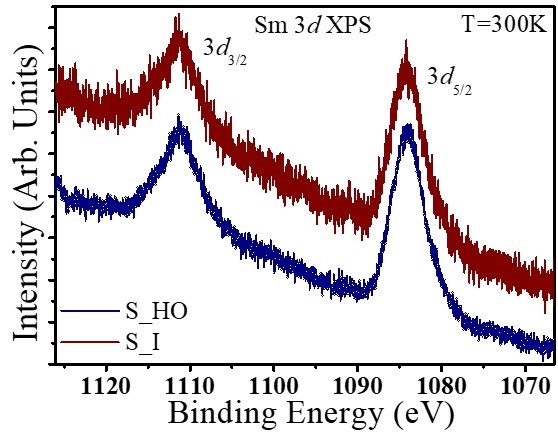}
\caption{Experimentally observed Sm $ 3d $ core level photo emission spectra measured at T=300 K for the SNMO thin films having different anti-site disorder densities. To have better visualization spectra are vertically translated here.}\label{sm3dxps}
\end{figure*} 

\begin{figure*}[]\renewcommand{\thefigure}{S\arabic{figure}}
\centering
\includegraphics[angle=0,width=1.0\textwidth]{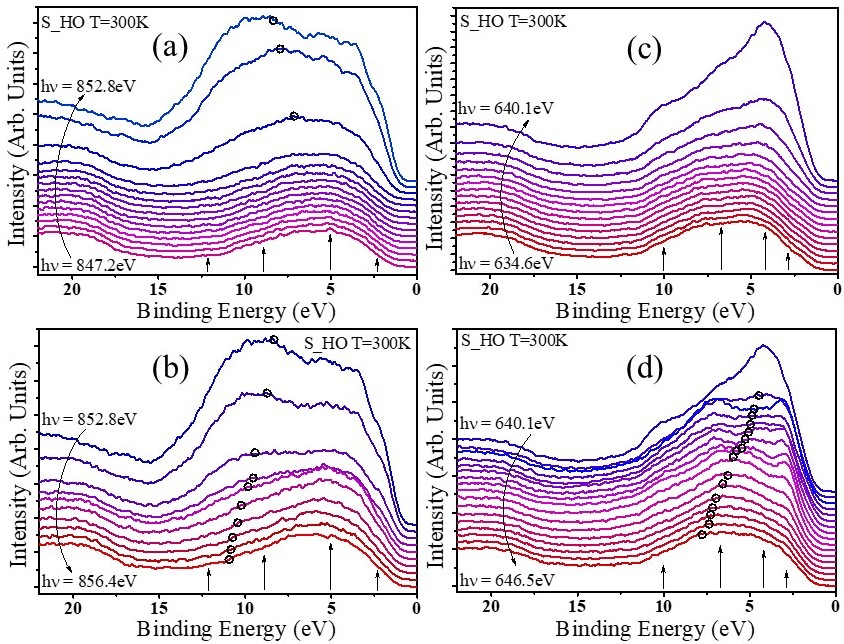}
\caption{Valence band photo emission spectra recorded at T=300K with varying incident photon energies across Ni/Mn $ 2p_{3/2} \rightarrow 3d $ photo absorption regime for S$ \_ $HO film. (a): Pre resonance of Ni $ L_{3} $ threshold. (b): Post resonance of Ni $ L_{3} $ threshold. (c): Pre resonance of Mn $ L_{3} $ threshold. (d): Post resonance of Mn $ L_{3} $ threshold. To have clear visualization spectra are vertically translated here.}\label{shorespes300k}
\end{figure*}

\begin{figure*}[]\renewcommand{\thefigure}{S\arabic{figure}}
\centering
\includegraphics[angle=0,width=1.0\textwidth]{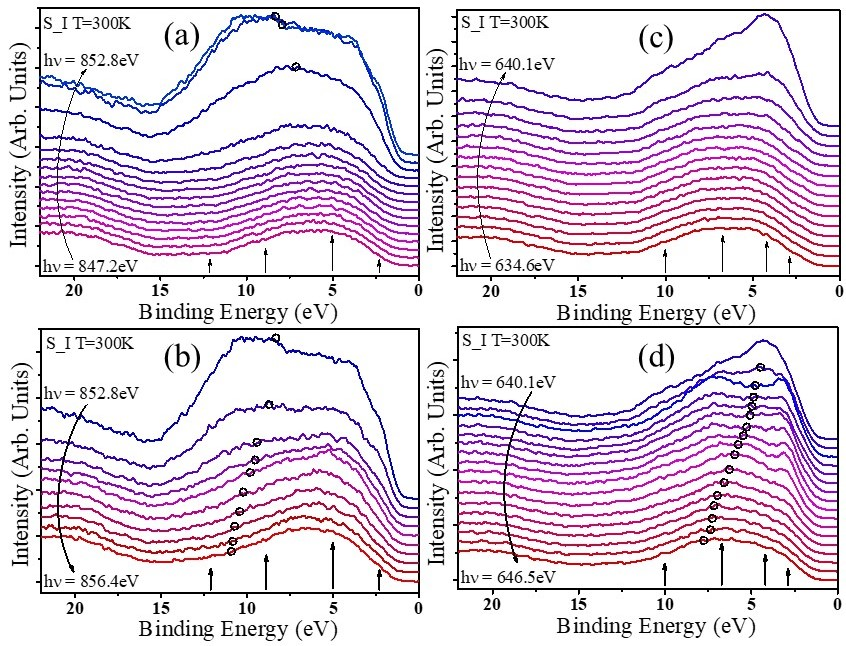}
\caption{Valence band photo emission spectra recorded at T=300K with varying incident photon energies across Ni/Mn $ 2p_{3/2} \rightarrow 3d $ photo absorption regime for S$ \_ $I film.  (a): Pre resonance of Ni $ L_{3} $ threshold. (b): Post resonance of Ni $ L_{3} $ threshold. (c): Pre resonance of Mn $ L_{3} $ threshold. (d): Post resonance of Mn $ L_{3} $ threshold. To have clear visualization spectra are vertically translated here.}\label{sirespes300k}
\end{figure*}

\begin{figure*}[]\renewcommand{\thefigure}{S\arabic{figure}}
\centering
\includegraphics[angle=0,width=1.0\textwidth]{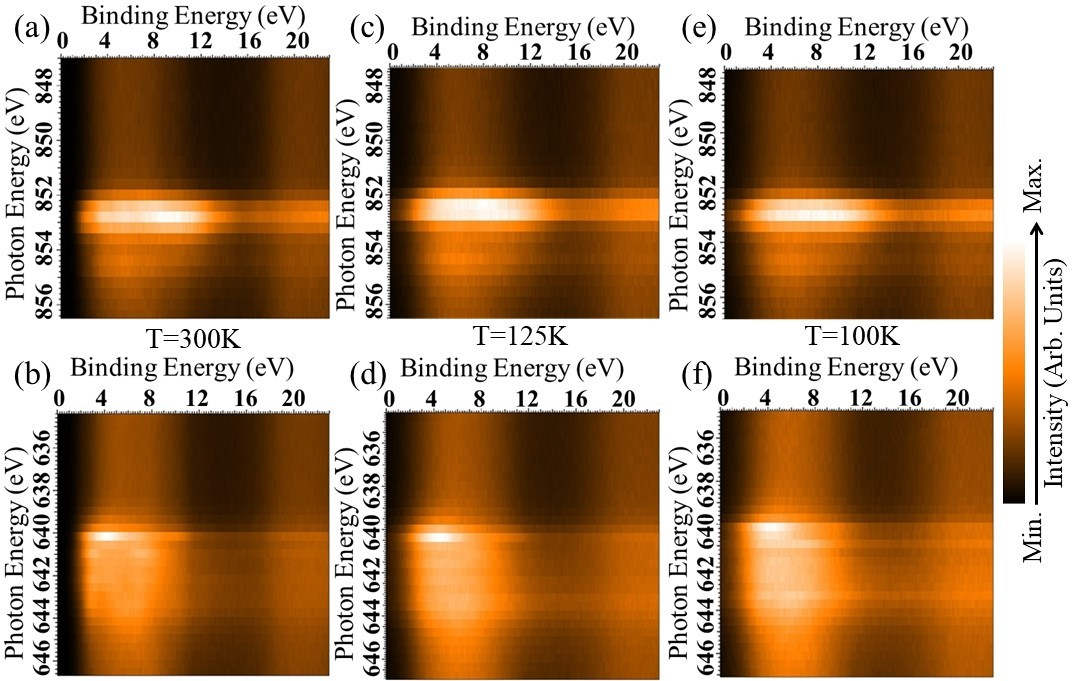}
\caption{Resonance photo emission maps acquired at different temperatures for S$ \_ $HO film. (a): At T=300K across Ni $ 2p_{3/2} \rightarrow 3d $ threshold, (b): At T=300K across Mn $ 2p_{3/2} \rightarrow 3d $ threshold, (c): At T=125K across Ni $ 2p_{3/2} \rightarrow 3d $ threshold, (d) At T=125K across Mn $ 2p_{3/2} \rightarrow 3d $ threshold, (e): At T=100K across Ni $ 2p_{3/2} \rightarrow 3d $ threshold, (f): At T=100K across Mn $ 2p_{3/2} \rightarrow 3d $ threshold.}\label{respesmapvst}
\end{figure*}

\begin{figure*}[]\renewcommand{\thefigure}{S\arabic{figure}}
\centering
\includegraphics[angle=0,width=1.0\textwidth]{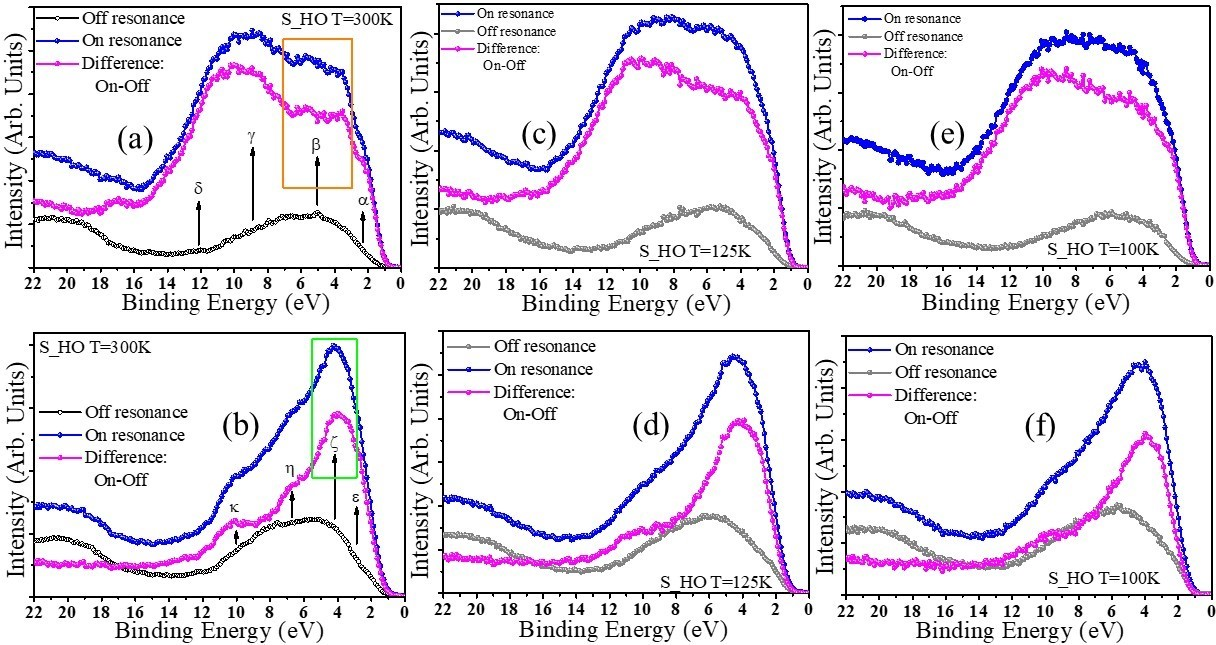}
\caption{On, off resonance and on-off difference spectra for S$ \_ $HO film measured at different temperatures. (a): At T=300K across Ni $ 2p_{3/2} \rightarrow 3d $ threshold. (b): At T=300K across Mn $ 2p_{3/2} \rightarrow 3d $ threshold. (c): At T=125K across Ni $ 2p_{3/2} \rightarrow 3d $ threshold. (d): At T=125K across Mn $ 2p_{3/2} \rightarrow 3d $ threshold. (e): At T=100K across Ni $ 2p_{3/2} \rightarrow 3d $ threshold. (f): At T=100K across Mn $ 2p_{3/2} \rightarrow 3d $ threshold. }\label{onoffrespesvst}
\end{figure*}

\begin{figure*}[]\renewcommand{\thefigure}{S\arabic{figure}}
\centering
\includegraphics[angle=0,width=0.5\textwidth]{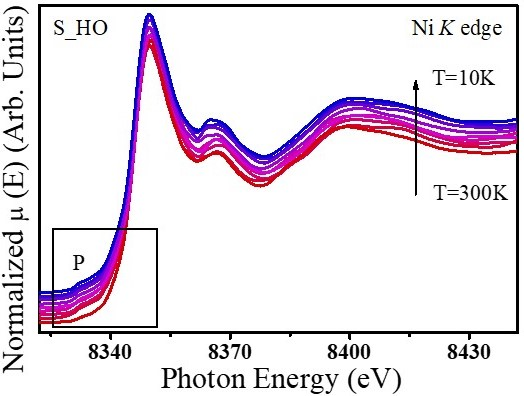}
\caption{(a): Thermal evolution of Ni $ K $ near edge X-ray absorption spectra measured for S$ \_ $HO thin film. The pre-edge features are highlighted by box `P'.}\label{nikt}
\end{figure*}

\end{document}
