# Supplementary material for: Robust electronic and tunable magnetic states in Sm$ _{2} $NiMnO$ _{6} $ ferromagnetic insulator
Source: arXiv:2204.08843 source file (2022-04-19)
Supplement: Supplementary file 2 [file Supplementary_Informations_SNMO_film_E_V2.pdf]

# Supplementary Information:

## Robust electronic and tunable magnetic states in $\text{Sm}_2\text{NiMnO}_6$ ferromagnetic insulator

S. Majumder<sup>a</sup>, M. Tripathi<sup>a</sup>, I. Píš<sup>b,c</sup>, S. Nappini<sup>c</sup>, P. Rajput<sup>d</sup>, S. N. Jha<sup>d</sup>, R. J. Choudhary<sup>a</sup>, and D. M. Phase<sup>a</sup>

<sup>a</sup>UGC DAE Consortium for Scientific Research, Indore 452001, India

<sup>b</sup>Elettra Sincrotrone Trieste S.C.p.A., S.S. 14-km 163.5, 34149 Basovizza, Trieste, Italy

<sup>c</sup>IOM CNR, Laboratorio TASC, S.S. 14-km 163.5, 34149 Basovizza, Trieste, Italy

<sup>d</sup>Beamline Development and Application Section, Bhabha Atomic Research Centre, Mumbai 400085, India

E-mail: \*ram@csr.res.in

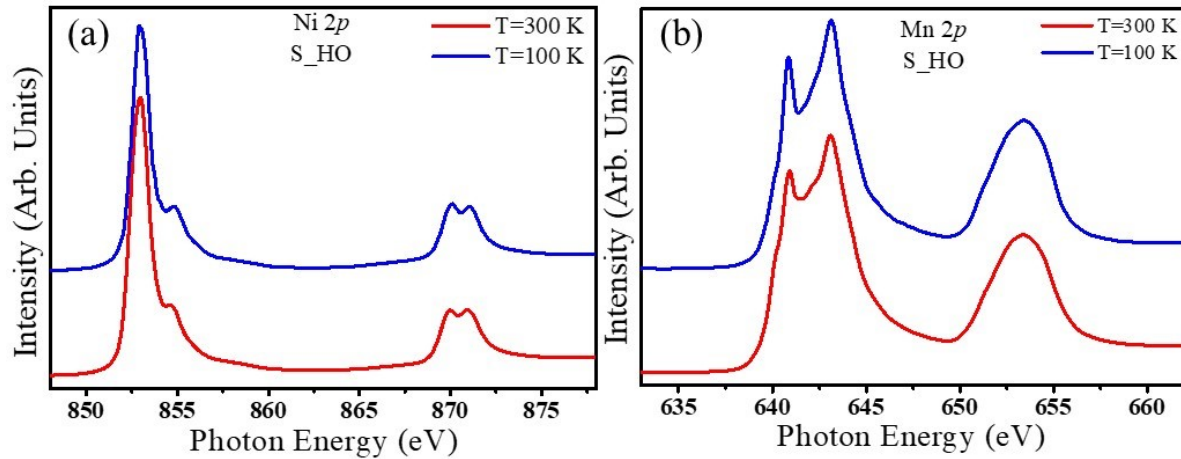

**Figure S1.** Experimentally observed photo absorption spectra measured for S\_HO sample at T=300 K, 100 K across (a): Ni and (b): Mn  $L_{3,2}$  edges. To have better visualization spectra are vertically translated here.

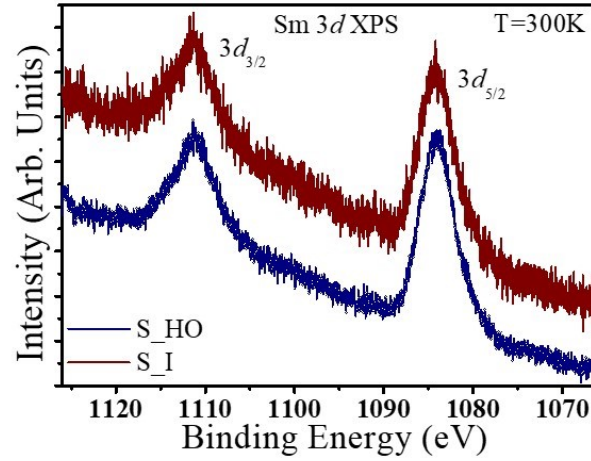

**Figure S2.** Experimentally observed Sm 3d core level photo emission spectra measured at T=300 K for the SNMO thin films having different anti-site disorder densities. To have better visualization spectra are vertically translated here.

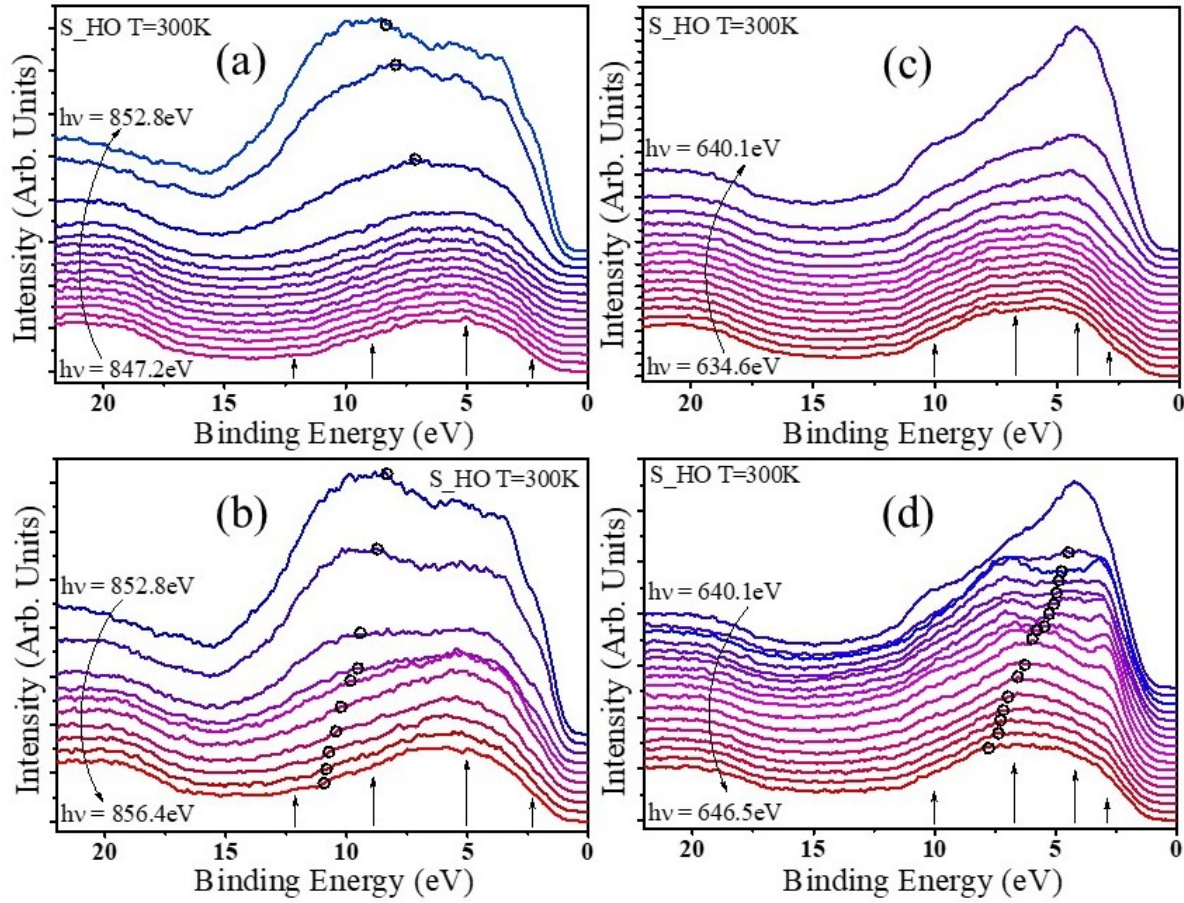

**Figure S3.** Valence band photo emission spectra recorded at T=300K with varying incident photon energies across Ni/Mn  $2p_{3/2} \rightarrow 3d$  photo absorption regime for S\_HO film. (a): Pre resonance of Ni  $L_3$  threshold. (b): Post resonance of Ni  $L_3$  threshold. (c): Pre resonance of Mn  $L_3$  threshold. (d): Post resonance of Mn  $L_3$  threshold. To have clear visualization spectra are vertically translated here.

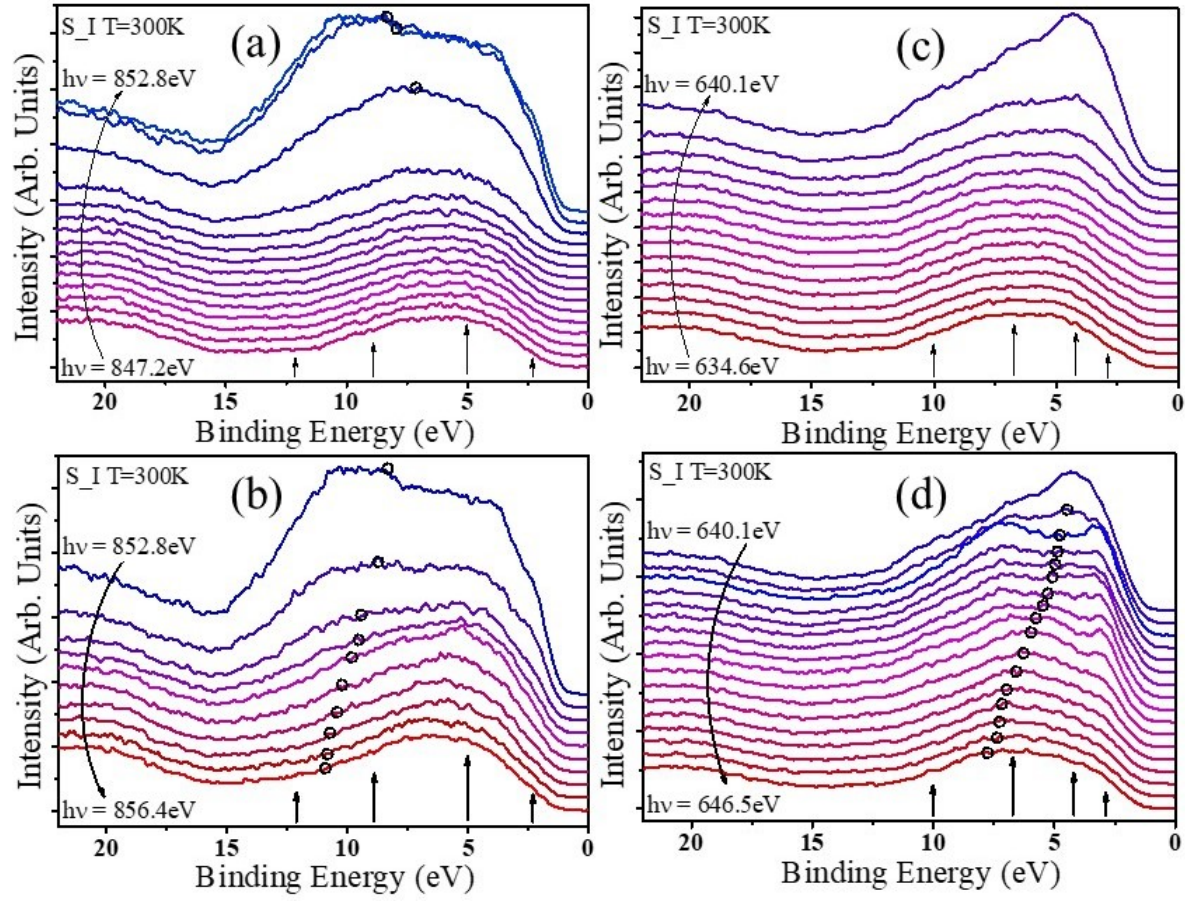

**Figure S4.** Valence band photo emission spectra recorded at  $T=300\text{K}$  with varying incident photon energies across Ni/Mn  $2p_{3/2} \rightarrow 3d$  photo absorption regime for S.I film. (a): Pre resonance of Ni  $L_3$  threshold. (b): Post resonance of Ni  $L_3$  threshold. (c): Pre resonance of Mn  $L_3$  threshold. (d): Post resonance of Mn  $L_3$  threshold. To have clear visualization spectra are vertically translated here.



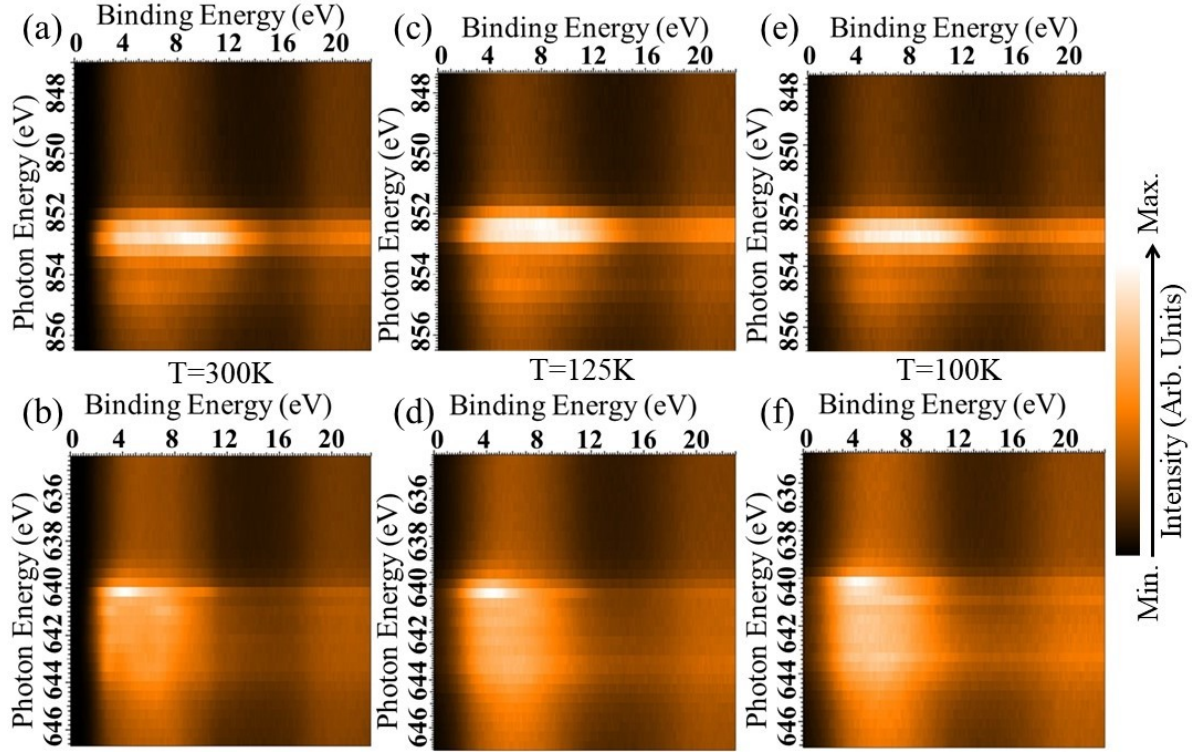

**Figure S5.** Resonance photo emission maps acquired at different temperatures for S.HO film. (a): At T=300K across Ni  $2p_{3/2} \rightarrow 3d$  threshold, (b): At T=300K across Mn  $2p_{3/2} \rightarrow 3d$  threshold, (c): At T=125K across Ni  $2p_{3/2} \rightarrow 3d$  threshold, (d) At T=125K across Mn  $2p_{3/2} \rightarrow 3d$  threshold, (e): At T=100K across Ni  $2p_{3/2} \rightarrow 3d$  threshold, (f): At T=100K across Mn  $2p_{3/2} \rightarrow 3d$  threshold.

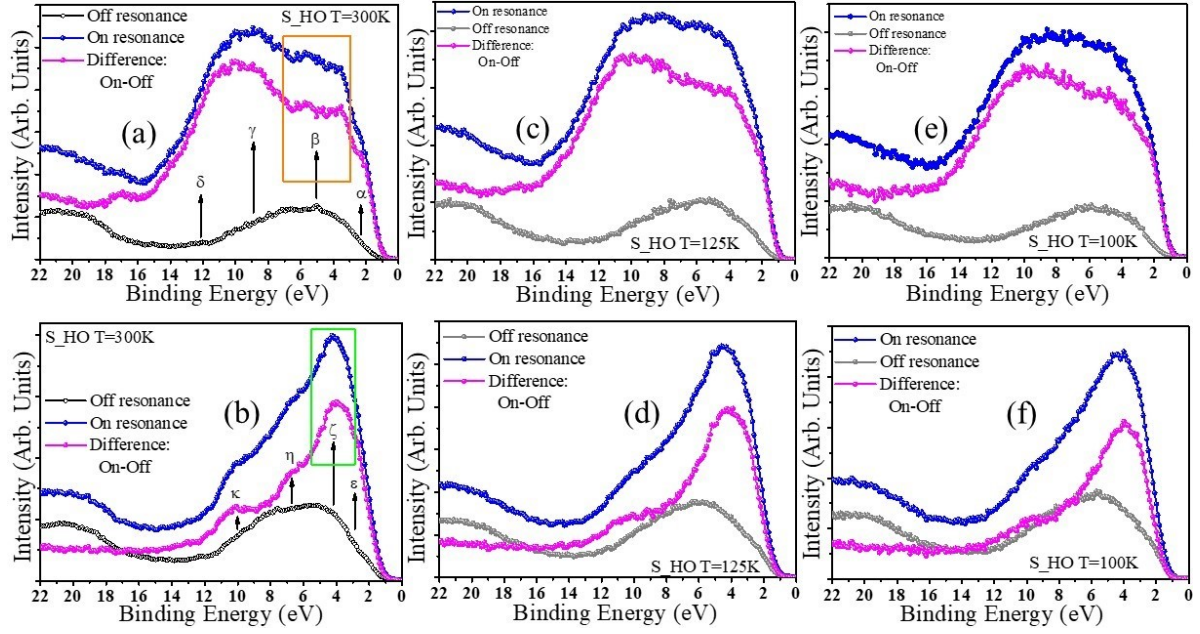

**Figure S6.** On, off resonance and on-off difference spectra for S\_HO film measured at different temperatures. (a): At  $T=300\text{K}$  across  $\text{Ni } 2p_{3/2} \rightarrow 3d$  threshold. (b): At  $T=300\text{K}$  across  $\text{Mn } 2p_{3/2} \rightarrow 3d$  threshold. (c): At  $T=125\text{K}$  across  $\text{Ni } 2p_{3/2} \rightarrow 3d$  threshold. (d): At  $T=125\text{K}$  across  $\text{Mn } 2p_{3/2} \rightarrow 3d$  threshold. (e): At  $T=100\text{K}$  across  $\text{Ni } 2p_{3/2} \rightarrow 3d$  threshold. (f): At  $T=100\text{K}$  across  $\text{Mn } 2p_{3/2} \rightarrow 3d$  threshold.

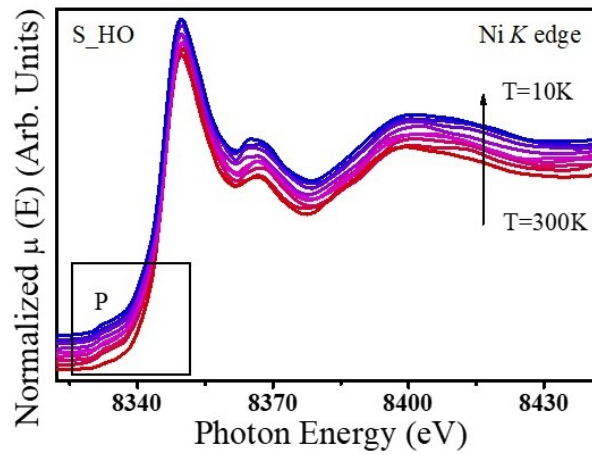

**Figure S7.** (a): Thermal evolution of Ni  $K$  near edge X-ray absorption spectra measured for S\_HO thin film. The pre-edge features are highlighted by box 'P'.
